# Supplementary material for: Learning to Solve PDE-constrained Inverse Problems with Graph Networks
Source: arXiv:2206.00711 source file (2022-06-01)
Supplement: Supplementary file 1 [file 6_appendix.tex]

\subsection{Two-Dimensional Scalar Wave Equation}
%%%%%%%%%%%%%%%%%%%%%%%%%%%%%%%%%%%%%%%%%%%%%%%%%%%%%%%%
\subsubsection{Dataset}
Dataset consist of 1100 training trajectories over 37 meshes, and 40 test trajectories over 3 meshes. For each mesh, we have a fish shape obstacle at the center obtained from the shape dataset \cite{shape_dataset}. The Dirichlet boundary condition is applied to all boundaries.  Ground truth trajectories are obtained using an open source FEM solver, FEniCs \cite{LoggMardalEtAl2012} on fine mesh with Euler method and first order elements. Supervised fields on coarse meshes and regular meshes are all interpolated from the simulation results on fine meshes. For every trajectory, we randomly sample an initial state, and a velocity distribution from the gaussian random field. The velocity distribution is threshold to binary. To satisfy the boundary conditions, the sampled initial state is decayed to 0 using the solution of Eikonal equation.
%%%%%%%%%%%%%%%%%%%%%%%%%%%%%%%%%%%%%%%%%%%%%%%%%%%%%%%%
\subsubsection{Prior newtork}
For the prior networks, $\prior_c$ or $\prior_u$, we use a multilayer perceptron (MLP) with 6 hidden layers, hidden features of size $256$, and positional encoding \cite{tancik2020fourier}. ReLU nonlinearity is used at all intermediate layers and sigmoid is used at the final layer. Input latent code is of size $64$. During the training, the dataset is normalized to be between $[0,1]$. We train the network with ADAM optimizer \cite{kingma2014adam} for 1500 epochs with batch size of 32, learning rate of 5e-4. For each sample, we random sample 900 points and add random noise to the coordinates for better generalization. The loss function is \eqref{loss_prior}, where $\sigma=0.01$. 
%%%%%%%%%%%%%%%%%%%%%%%%%%%%%%%%%%%%%%%%%%%%%%%%%%%%%%%%
\subsubsection{Hyperparameters for learned simulators}
\paragraph{U-Net}
For U-Net, we adopt the architecture in \cite{thuerey:2020}. Input of the network consist of 3 channels, $[u,u', \text{mask}]$, where the "mask" indicates the simulation domain. We adjust the network size so that the total number of parameters matches the total number of parameters used in GNN. We train the network for 500 epochs with the ADAM optimizer \cite{kingma2014adam}, learning rate 0.0004 and batch size 10.
\paragraph{GNN}
For GNN, we adopt the architecture in \cite{pfaff2020learning}. The input edge features consist of distance between nodes and normalized direction between nodes. The input node features consist of $[u,u',\text{node type}]$, where node type is a one-hot vector that is $[0,1]$ on the boundary, or $[1,0]$ off boundary. The hidden features size of each MLP is $256$ and the total number of message passing steps is 10. We train the network using the ADAM optimizer \cite{kingma2014adam} with learning rate 1e-4 exponentially decay to 1e-8 over 500 epochs. 
%%%%%%%%%%%%%%%%%%%%%%%%%%%%%%%%%%%%%%%%%%%%%%%%%%%%%%%%
\subsubsection{Qualitative Comparisons}
Here, we show more qualitative comparisons for initial state recovery, \figref{wave_compare_init}, and full-waveform inversion task, \figref{wave_compare_density}, for the wave equation. 
\begin{figure}[h]
    \centering
    \includegraphics[width=0.5\textwidth]{image/appex/wave_init_comparison_labeled.png}
    \caption{Sample comparisons for initial state recovery results with the wave equation.}
    \label{fig:wave_compare_init}
\end{figure}
\begin{figure}[h]
    \centering
    \includegraphics[width=0.5\textwidth]{image/appex/wave_density_comparison_labeled.png}
    \caption{Sample comparisons for full-waveform inversion results with the wave equation.}
    \label{fig:wave_compare_density}
\end{figure}
%%%%%%%%%%%%%%%%%%%%%%%%%%%%%%%%%%%%%%%%%%%%%%%%%%%%%%%%5
\clearpage
\newpage
\subsection{Two-Dimensional Incompressible Navier Stokes
Equation}
%%%%%%%%%%%%%%%%%%%%%%%%%%%%%%%%%%%%%%%%%%%%%%%%%%%%%%%%
\subsubsection{Dataset}
Fluid dataset consist of 850 training trajectories on 55 meshes, and 50 test trajectories on 5 meshes. Ground truth trajectories are obtained through simulation using open source FEM solver, FEniCs \cite{LoggMardalEtAl2012} with fine meshes using Chorin’s method. For every trajectory, we randomly sample an initial velocity field, $\uxy$. The first 1000 steps of iteration are treated as warm start and is not used during the training.   
%%%%%%%%%%%%%%%%%%%%%%%%%%%%%%%%%%%%%%%%%%%%%%%%%%%%%%%%
\subsubsection{Prior newtork}
For prior networks, $\prior_\uxy$, we use a multilayer perceptron (MLP) with 6 hidden layers, hidden features of size $256$, and positional encoding \cite{tancik2020fourier}. ReLU nonlinearity is used at all intermediate layers and at the outmost layer. Input latent code is of size $128$. The skip connection is also adopted here, i.e. the input latent code is concatenated to the 3rd and 5th layer. During the training, the dataset is normalized to be between $[0,1]$. We train the network with the ADAM optimizer \cite{kingma2014adam} for 1500 epochs with batch size of 32 and learning rate of 5e-4. For each sample, we random sample 4000 points and add random noise to the coordinates for better generalization. The loss function is \eqref{loss_prior}, where $\sigma=0.01$. 
%%%%%%%%%%%%%%%%%%%%%%%%%%%%%%%%%%%%%%%%%%%%%%%%%%%%%%%%
\subsubsection{Hyperparameters for learned simulators}
\paragraph{U-Net}
For U-Net, we adopt the architecture in \cite{thuerey:2020}. Input of network consist of 3 channels, $[u_x,u_y,\text{mask}]$, where the "mask" indicates the simulation domain. We adjust the network size so that the total number of parameters matches the total number of parameters used in the GNN. To train the model, we train for 500 epochs with the ADAM
optimizer \cite{kingma2014adam}, learning rate 0.0004 and batch size 128. 
\paragraph{GNN}
For GNN, we adopt the architecture in \cite{pfaff2020learning}. The input edge features consist of distance between nodes and normalized direction between nodes. The input node features consist of $[u_x,u_y,\text{node type}]$, where node type is a one-hot vector indicates if the node is at the inlet, outlet, cylinder boundary, wall boundaries, or out of the boundary. The hidden features size of each MLP is $128$ and total number of message passing steps is 15. We train the network with the ADAM optimizer \cite{kingma2014adam} with learning rate 1e-4 exponentially decay to 1e-8 over 500 epochs. 
%%%%%%%%%%%%%%%%%%%%%%%%%%%%%%%%%%%%%%%%%%%%%%%%%%%%%%%%
\subsubsection{Fine tuning}
\begin{table}[h]
\centering
\begin{tabular}{l|cccc}\toprule
\textbf{Forward Model}	  & \multicolumn{4}{c}{\textbf{Fluid Data Assimilation}} \\
                          & \multicolumn{2}{c}{\textbf{without Fine-tuning}} & \multicolumn{2}{c}{\textbf{with Fine-tuning}} \\
                          & MSE ($V_x$)      & MSE ($V_y$)           & MSE ($V_x$) & MSE ($V_y$) 		\\\midrule
FEM  (Irr. C.)            & \textbf{5.58e-3} & \textbf{2.83e-3}    & \textbf{4.46e-3} & \underline{1.94e-3} \\
U-Net (Reg. C.)           & 1.21e-2   & 6.17e-3                      & {1.02e-3}	    & {5.40e-3}	 \\
U-Net (Reg. F.)           & \underline{8.64e-3}   & \underline{4.04e-3}                      & {7.974e-3} 	& {3.31e-3} \\
GNN  (Irr. C.)            & 9.87e-3   & 4.19e-3   & {\underline{6.55e-3}}& {\textbf{1.86e-3}}\\\bottomrule
\end{tabular}
\label{table:fluid}
\caption{Fluid assimilation results averaged over 50 test samples on 5 unseen meshes. Here, each flow clip consist of 10 GNN time steps. We taking measurement of the velocity $[u_x,u_y]$ every 2 time steps using 50 sampled sensors. Here we compare the with fine-tuning and the without fine-tuning approach. We observe that for with fine-tuning approach, we achieve lower MSE.} 
\end{table}
%%%%%%%%%%%%%%%%%%%%%%%%%%%%%%%%%%%%%%%%%%%%%%%%%%%%%%%%    
\subsubsection{Qualitative Comparisons}
In \figref{fluid_compare}, we show qualitative comparisons for the flow assimilation task. 
\begin{figure}[h]
    \centering
    \includegraphics[width=0.8\textwidth]{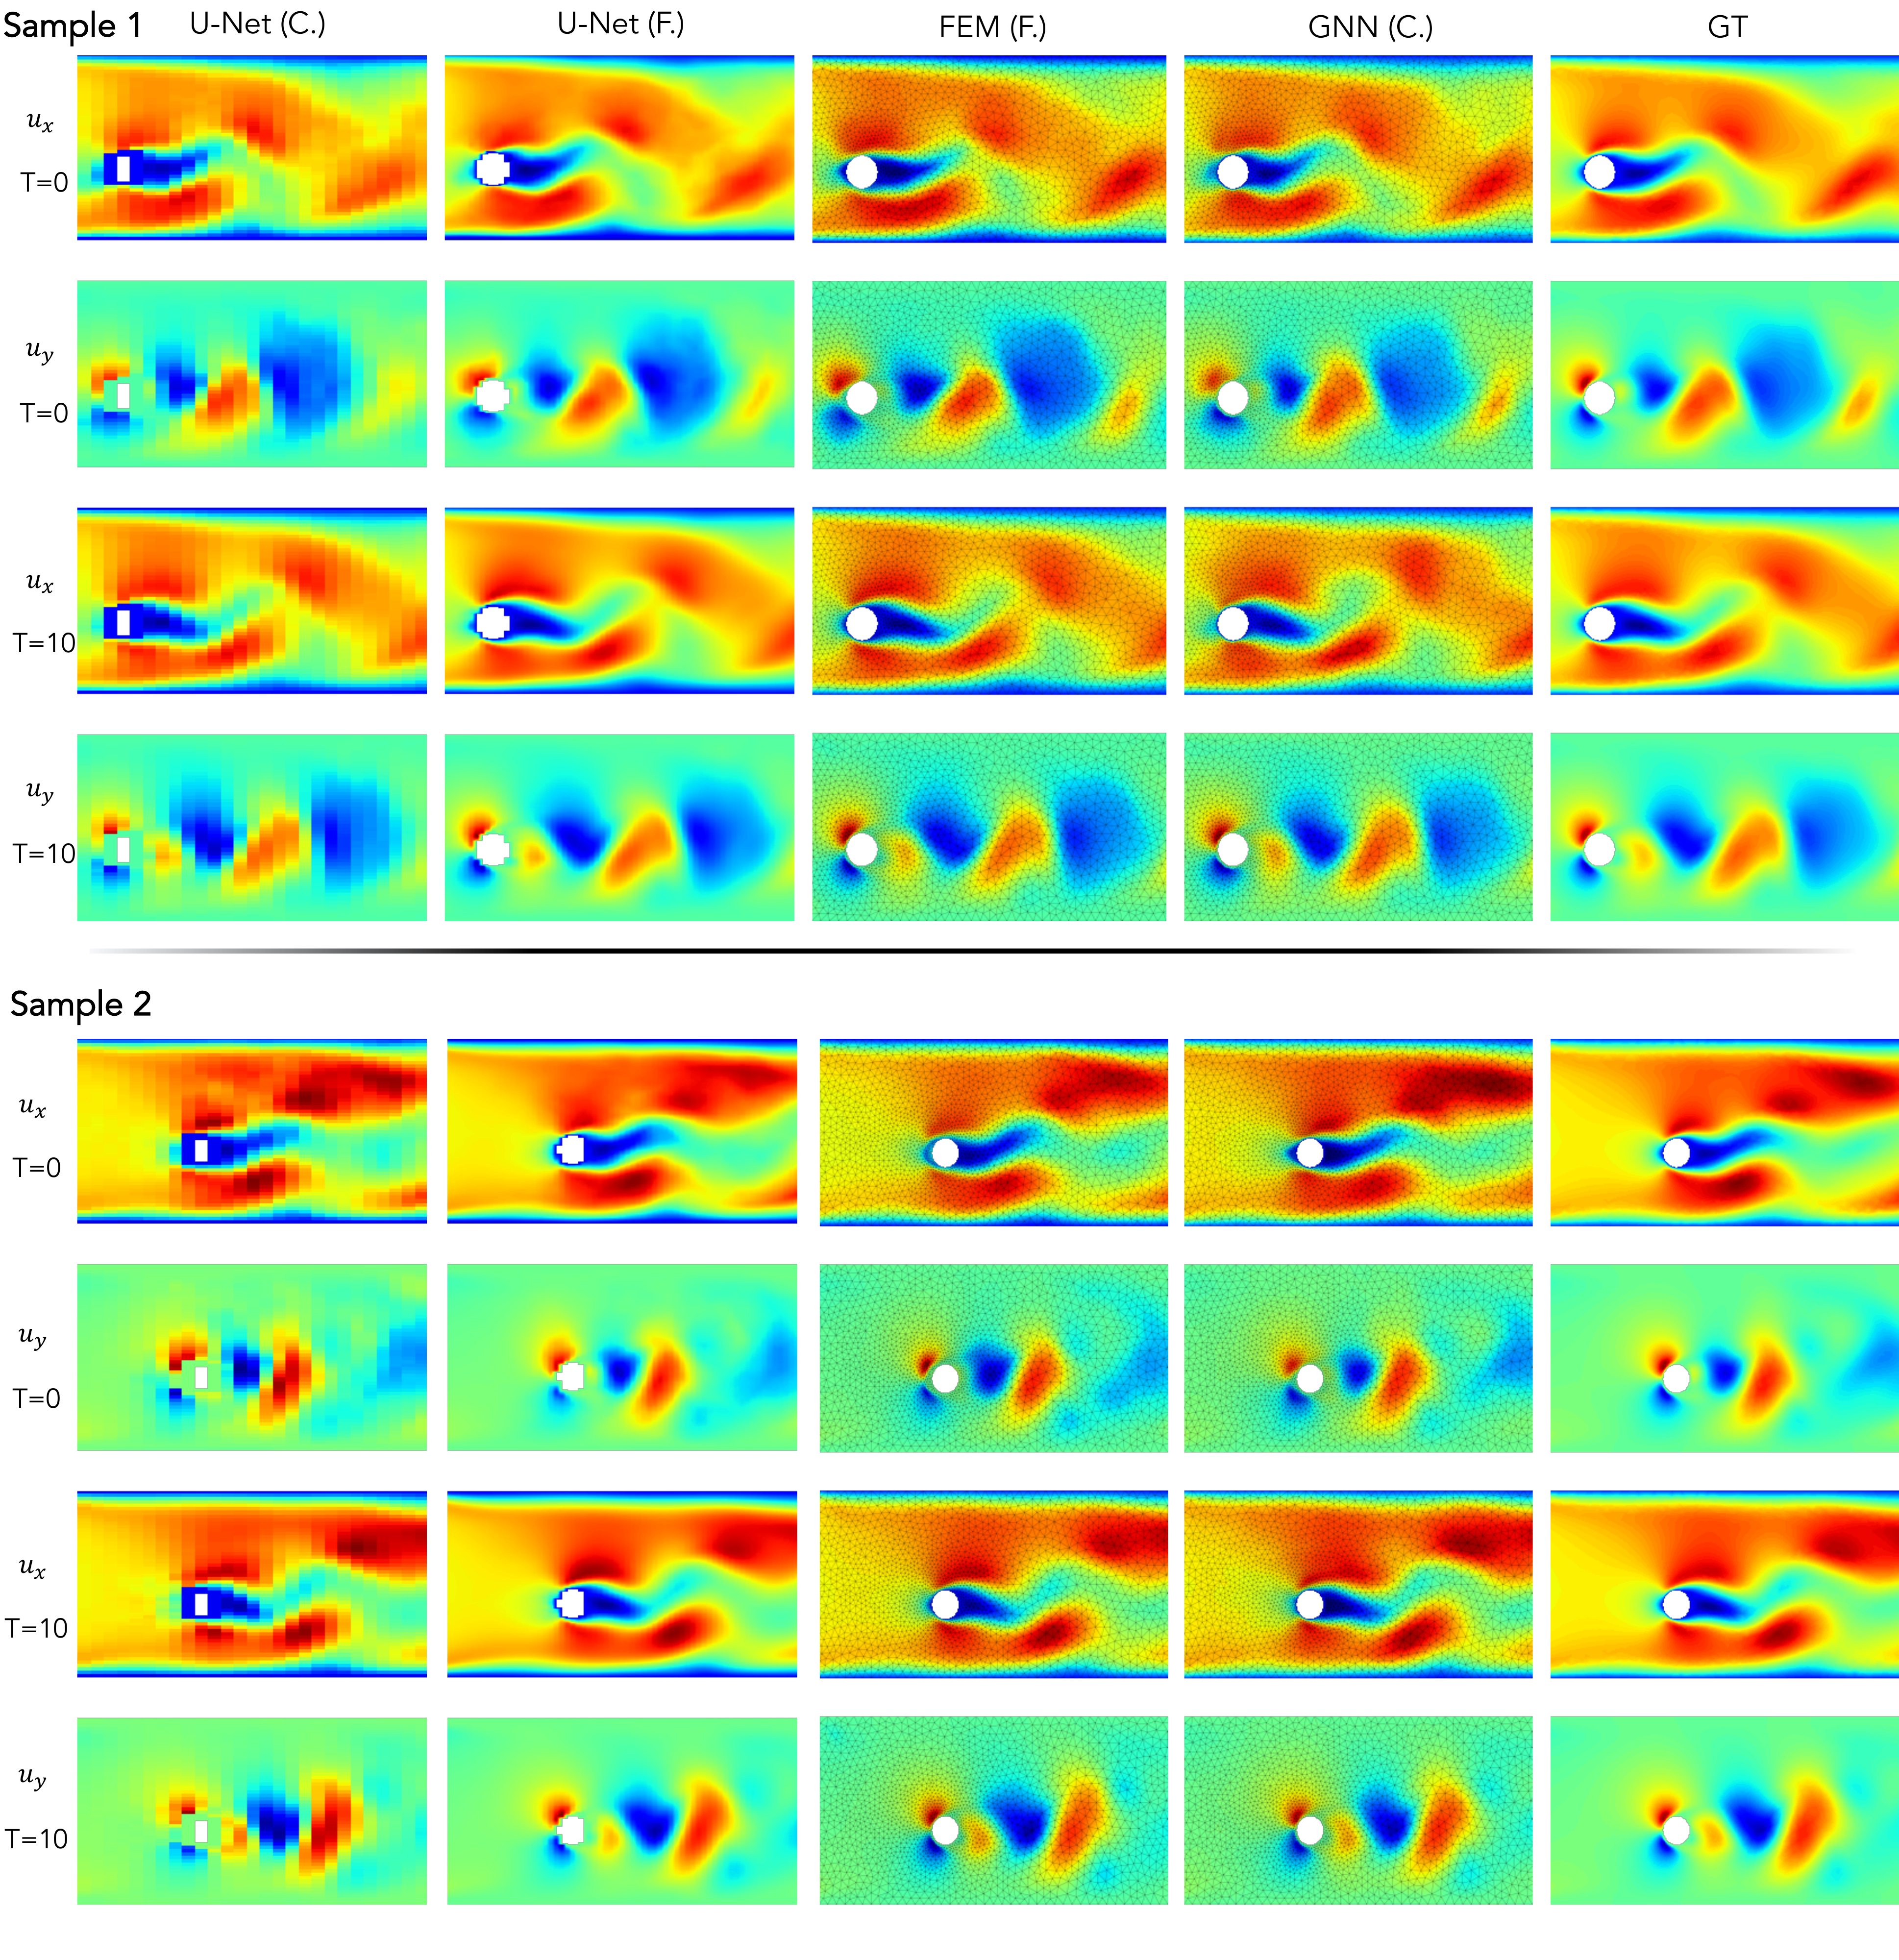}
    \caption{Sample comparisons for flow assimilation task.}
    \label{fig:fluid_compare}
\end{figure}
